# Supplementary material for: One Layer's Trash is Another Layer's Treasure: Adaptive Layer-wise Visual Token Selection in LVLMs
Source: arXiv:2606.14277 source file (2026-06-12)
Supplement: Supplementary file 1 [file X_suppl.tex]

\clearpage
\setcounter{page}{1}
\maketitlesupplementary
\appendix  % 自行添加

\section{Benchmark Details}
\label{sec:benchmark details}
\begin{itemize}
\item \textbf{AI2D}~\cite{kembhavi2016diagram} focuses on diagram interpretation and reasoning, comprising over 5,000 grade school science diagrams with comprehensive annotations. Each diagram is associated with multiple-choice questions, totaling more than 15,000 questions across the dataset. This benchmark is specifically designed to evaluate models' ability to understand complex visual structures, parse spatial relationships, and perform domain-specific semantic reasoning about scientific concepts depicted in educational diagrams.

\item \textbf{POPE}~\cite{li2023evaluating} assesses object hallucination in large vision-language models by formulating evaluation as a binary classification task using simple yes-or-no questions. Built on the MS COCO validation set, we evaluate on 500 randomly selected images with 6 questions per image, totaling 3,000 question-answer pairs. Three sampling strategies are employed: random, popular (frequently appearing objects), and adversarial (frequently co-occurring objects). Performance is measured using accuracy, precision, recall, and F1 score.

\item \textbf{TextVQA}~\cite{singh2019towards} addresses visual question answering requiring reading and reasoning about text in images, containing 45,336 questions on 28,408 images sourced from the Open Images dataset. Each question is annotated with 10 human-provided answers, with the dataset split into 34,602 training, 5,000 validation, and 5,734 test questions. The benchmark specifically tests models' ability to detect, recognize, and reason about textual content embedded within natural scene images.

\item \textbf{OKVQA}~\cite{marino2019ok} features 14,055 questions where image content alone is insufficient for answering, requiring external knowledge resources. Questions are collected on COCO images, with 9,009 training and 5,046 test samples, each accompanied by 10 answer annotations. The dataset spans 10 knowledge categories including science, history, sports, and geography. We follow the standard evaluation protocol using the VQA accuracy metric, comparing predicted answers against human annotations.

\item \textbf{VizWiz}~\cite{gurari2018vizwiz} is a goal-oriented VQA dataset comprising over 31,000 visual questions from blind users who captured images via mobile phones and recorded spoken queries. Each image is annotated with 10 crowdsourced answers. The dataset presents unique challenges including poor image quality (blur, lighting issues, obstructed views) and conversational question styles. We evaluate on the test split using the standard VQA accuracy metric.

\item \textbf{COCO Caption}~\cite{lin2014microsoft} is built upon the MS COCO dataset, which contains 328,000 images depicting complex everyday scenes with common objects in natural contexts. The dataset comprises 91 object categories and 2.5 million labeled instances. Each image is paired with five human-generated descriptive captions collected via crowdsourcing. Following standard practice, we report CIDEr as the primary captioning metric for performance assessment.

\item \textbf{NoCaps}~\cite{agrawal2019nocaps} is a novel object captioning benchmark consisting of 15,100 images from Open Images with 166,100 human-generated captions. Each image contains 10 reference captions plus one human baseline caption. Test images are divided into in-domain, near-domain, and out-of-domain subsets based on object category overlap with COCO. We evaluate on all three splits using the CIDEr metric.

\item \textbf{RealWorldQA} is a real-world visual understanding benchmark containing 765 images captured from vehicles and diverse real-world settings. Each image is paired with a question requiring visual reasoning and a verifiable answer. Questions span object recognition, spatial relationships, directional understanding, and scene comprehension. We report accuracy on the full test set.
\end{itemize}

% ------------------------------
\section{Implementation Details}
Experiments with LLaVA-1.5-7B~\cite{liu2024improved}, LLaVA-NeXT-7B~\cite{liu2024llavanext}, and Qwen2.5-VL-3B-Instruct~\cite{bai2025qwen2} models are conducted on a single NVIDIA GeForce RTX 4090 GPU. Experiments with the LLaVA-1.5-13B model are conducted on a single NVIDIA A100-40G GPU. The implementation is carried out in Python
3.10, utilizing PyTorch 2.1.2 and CUDA 12.2. The inference follows the evaluation settings of the LMMs-Eval framework~\cite{zhang2025lmms}.

% ------------------------------
\section{LLaVA-1.5-13B Detailed Results}
% 表格
\begin{table*}[t]
    \caption{Performance comparison of LLaVA-1.5-13B under different token reduction ratios. ``Avg.'' refers to the average performance across 8 benchmarks. Best results are shown in \textbf{bold}.}
    \label{tab:appendix_llava_1.5_13b}
    
    \centering
    \begin{tabular}{l|cccccccc|c}
    \toprule
    \textbf{Method} & \textbf{AI2D} & \textbf{POPE} & \textbf{VQA}$^{\text{Text}}$ & \textbf{OKVQA} & \textbf{VizWiz} & \textbf{COCO} & \textbf{NoCaps} & \textbf{RealWorld} & \textbf{Avg.} \\
    \midrule
    \multicolumn{10}{c}{\textit{Upper Bound, 576 Tokens (100\%)}} \\
    \midrule
    LLaVA-1.5-13B & 59.26 & 85.92 & 61.26 & 58.24 & 56.60 & 115.48 & 109.32 & 55.29 & 100.00\% \\
    \midrule
    \multicolumn{10}{c}{\textit{Retain 192 Tokens ($\downarrow$ 67\%)}} \\
    \midrule
    FastV {\footnotesize\textit{(ECCV-24)}} & 58.61 & 82.68 & 60.52 & 56.89 & 57.05 & 114.61 & 107.96 & 54.90 & 98.71\% \\
    VTW {\footnotesize\textit{(AAAI-25)}} & 59.42 & 82.24 & 54.69 & 44.76 & 50.66 & 82.40 & 67.05 & 53.73 & 85.19\% \\
    PDrop {\footnotesize\textit{(CVPR-25)}} & 57.64 & 84.77 & 59.46 & 58.11 & 55.65 & 113.76 & 107.08 & 52.81 & 97.88\% \\
    DART {\footnotesize\textit{(EMNLP-25)}} & 58.94 & 84.02 & 60.16 & 57.13 & \textbf{57.28} & 115.19 & 108.53 & \textbf{55.03} & 99.16\% \\
    \textbf{ALVTS (\textit{Ours})} & \textbf{59.52} & \textbf{85.79} & \textbf{60.62} & \textbf{58.12} & 56.61 & \textbf{116.19} & \textbf{108.96} & \textbf{55.03} & \textbf{99.86\%} \\
    \midrule
    \multicolumn{10}{c}{\textit{Retain 128 Tokens ($\downarrow$ 78\%)}} \\
    \midrule
    FastV {\footnotesize\textit{(ECCV-24)}} & 57.71 & 77.90 & 59.61 & 55.70 & \textbf{57.35} & 112.24 & 105.99 & 52.42 & 96.41\% \\
    VTW {\footnotesize\textit{(AAAI-25)}} & 58.45 & 67.39 & 51.40 & 32.88 & 49.83 & 44.95 & 27.03 & 46.67 & 69.19\% \\
    PDrop {\footnotesize\textit{(CVPR-25)}} & 58.06 & 85.28 & 59.52 & \textbf{57.95} & 53.42 & 110.81 & 102.70 & 52.16 & 96.56\% \\
    DART {\footnotesize\textit{(EMNLP-25)}} & 58.81 & 81.71 & 59.03 & 55.77 & \textbf{57.35} & 112.88 & 106.62 & 53.20 & 97.41\% \\
    \textbf{ALVTS (\textit{Ours})} & \textbf{59.03} & \textbf{86.40} & \textbf{60.49} & 57.75 & 56.77 & \textbf{113.37} & \textbf{106.93} & \textbf{54.51} & \textbf{99.12\%} \\
    \midrule
    \multicolumn{10}{c}{\textit{Retain 64 Tokens ($\downarrow$ 89\%)}} \\
    \midrule
    FastV {\footnotesize\textit{(ECCV-24)}} & 57.74 & 69.32 & 56.16 & 52.01 & \textbf{57.35} & 103.64 & 96.65 & 50.33 & 91.20\% \\
    VTW {\footnotesize\textit{(AAAI-25)}} & 55.70 & 1.46 & 45.16 & 22.83 & 49.98 & 7.80 & 5.08 & 43.40 & 48.35\% \\
    PDrop {\footnotesize\textit{(CVPR-25)}} & 56.87 & 79.83 & 58.00 & 55.38 & 53.46 & 106.92 & 93.99 & 49.54 & 92.66\% \\
    DART {\footnotesize\textit{(EMNLP-25)}} & 57.61 & 75.52 & 55.90 & 52.70 & 57.25 & 108.44 & 102.16 & 53.33 & 93.98\% \\
    \textbf{ALVTS (\textit{Ours})} & \textbf{58.61} & \textbf{82.39} & \textbf{59.18} & \textbf{56.49} & 56.13 & \textbf{109.58} & \textbf{102.66} & \textbf{53.46} & \textbf{96.63\%} \\
    \bottomrule
    \end{tabular}
\end{table*}
\cref{tab:appendix_llava_1.5_13b} presents the detailed per-benchmark performance of LLaVA-1.5-13B under different token reduction ratios. At a 67\% reduction ratio, ALVTS attains 99.86\% average performance, outperforming all competing methods. Notably, ALVTS maintains robust performance even at an 89\% reduction ratio, achieving 96.63\% versus 91.20\% for FastV~\cite{chen2024image}. The method demonstrates particular strength on challenging benchmarks like COCO Caption and NoCaps, validating its effectiveness in preserving critical visual information under aggressive compression.

% ------------------------------
\section{More Results on Effects of Layer-wise Dynamic Token Selection}
% 表格
\begin{table}[t]
    \caption{Effectiveness of dynamic token selection mechanism on FastV algorithm.}
    \label{tab:appendix_fastv_dynamic}

    \begin{tabular*}{\columnwidth}{@{\extracolsep{\fill}} l|cccc}
    \toprule
    \small\textbf{Method} & \small\textbf{POPE} & \small\textbf{OKVQA} & \small\textbf{COCO} & \small\textbf{NoCaps} \\
    \midrule
    \multicolumn{5}{c}{\textit{Token Reduction ($\downarrow$ 67\%)}} \\
    \midrule
    FastV & 77.79 &	51.77 &	107.49 & 102.26 \\
    FastV \footnotesize(w/ dynamic) & 82.12 &	52.03 &	110.82 & 103.86 \\
    \midrule
    \multicolumn{5}{c}{\textit{Token Reduction ($\downarrow$ 78\%)}} \\
    \midrule
    FastV & 72.10 &	49.90 &	101.99 & 97.06 \\
    FastV \footnotesize(w/ dynamic) & 76.34 &	50.76 &	109.39 & 100.59 \\
    \midrule
    \multicolumn{5}{c}{\textit{Token Reduction ($\downarrow$ 89\%)}} \\
    \midrule
    FastV & 59.55 &	45.14 &	82.62 &	79.01 \\
    FastV \footnotesize(w/ dynamic) & 67.85 &	46.39 &	103.15 & 92.61 \\
    \bottomrule
    \end{tabular*}
\end{table}
To validate the generalization of our proposed layer-wise dynamic token selection mechanism, we conduct additional experiments by integrating this mechanism into the FastV baseline method. FastV originally performs one-time static pruning after the second layer of the LLM and maintains the same pruned token subset throughout all subsequent layers. Here, we augment FastV with our dynamic selection strategy, which allows each layer to independently select tokens based on layer-specific importance scores. As shown in \cref{tab:appendix_fastv_dynamic}, the results demonstrate consistent and substantial improvements across all compression settings. At a 67\% reduction ratio, incorporating dynamic selection brings notable gains on POPE (+4.33) and COCO Caption (+3.33). As the reduction ratio increases to 78\% and 89\%, the benefits of dynamic selection become even more pronounced. These results confirm that the layer-wise dynamic token selection mechanism is not specific to ALVTS but rather represents a general principle that can enhance existing token pruning methods.

% ------------------------------
\section{Ablation Study about Token Selector Rank}
% 表格
\begin{table}[t]
    \caption{Ablation study on token selector rank in LLaVA-1.5-7B. Avg. denotes the average performance across all benchmarks relative to the original model, and Overhead indicates the parameter overhead per decoder layer.}
    \label{tab:appendix_rank_choice}

    % 将表格内所有字体缩小一号
    \small
    % 稍微减小列间距，为内容和竖线腾出空间
    \setlength{\tabcolsep}{3pt}

    \begin{tabular*}{\columnwidth}{@{\extracolsep{\fill}} c|cccccc}
    \toprule
    \textbf{Rank} & \textbf{POPE} & \textbf{OKVQA} & \textbf{COCO} & \textbf{NoCaps} & \textbf{Avg.} & \textbf{Overhead} \\
    \midrule
    64 & 81.68 & 48.33 & 105.73 & 95.50 & 92.93\% & 0.5\% \\
    128 & 83.38 & 48.57 & 106.33 & 96.17 & 93.83\% & 1.0\% \\
    256 & 83.87 & 49.66 & 105.89 & 97.60 & 94.72\% & 2.0\% \\
    384 & 84.07 & 49.77 & 106.64 & 97.38 & 94.95\% & 3.0\% \\
    \bottomrule
    \end{tabular*}
\end{table}
To determine the optimal rank for the token selector, we evaluate ALVTS with different rank settings, as shown in \cref{tab:appendix_rank_choice}. We observe that increasing the rank from 64 to 256 brings notable performance improvements, with the average performance rising from 92.93\% to 94.72\%. However, further increasing the rank from 256 to 384 yields only marginal gains (94.72\% to 94.95\%), while the parameter overhead per decoder layer increases from 2\% to 3\%. Therefore, we select a rank of 256 for LLaVA-1.5-7B, as it provides an optimal balance between model performance and parameter efficiency.

% ------------------------------
\section{More Visualizations of Token Compression}
% 附录可视化结果图
\begin{figure*}[t]
  \centering
  \includegraphics[width=0.9\textwidth]{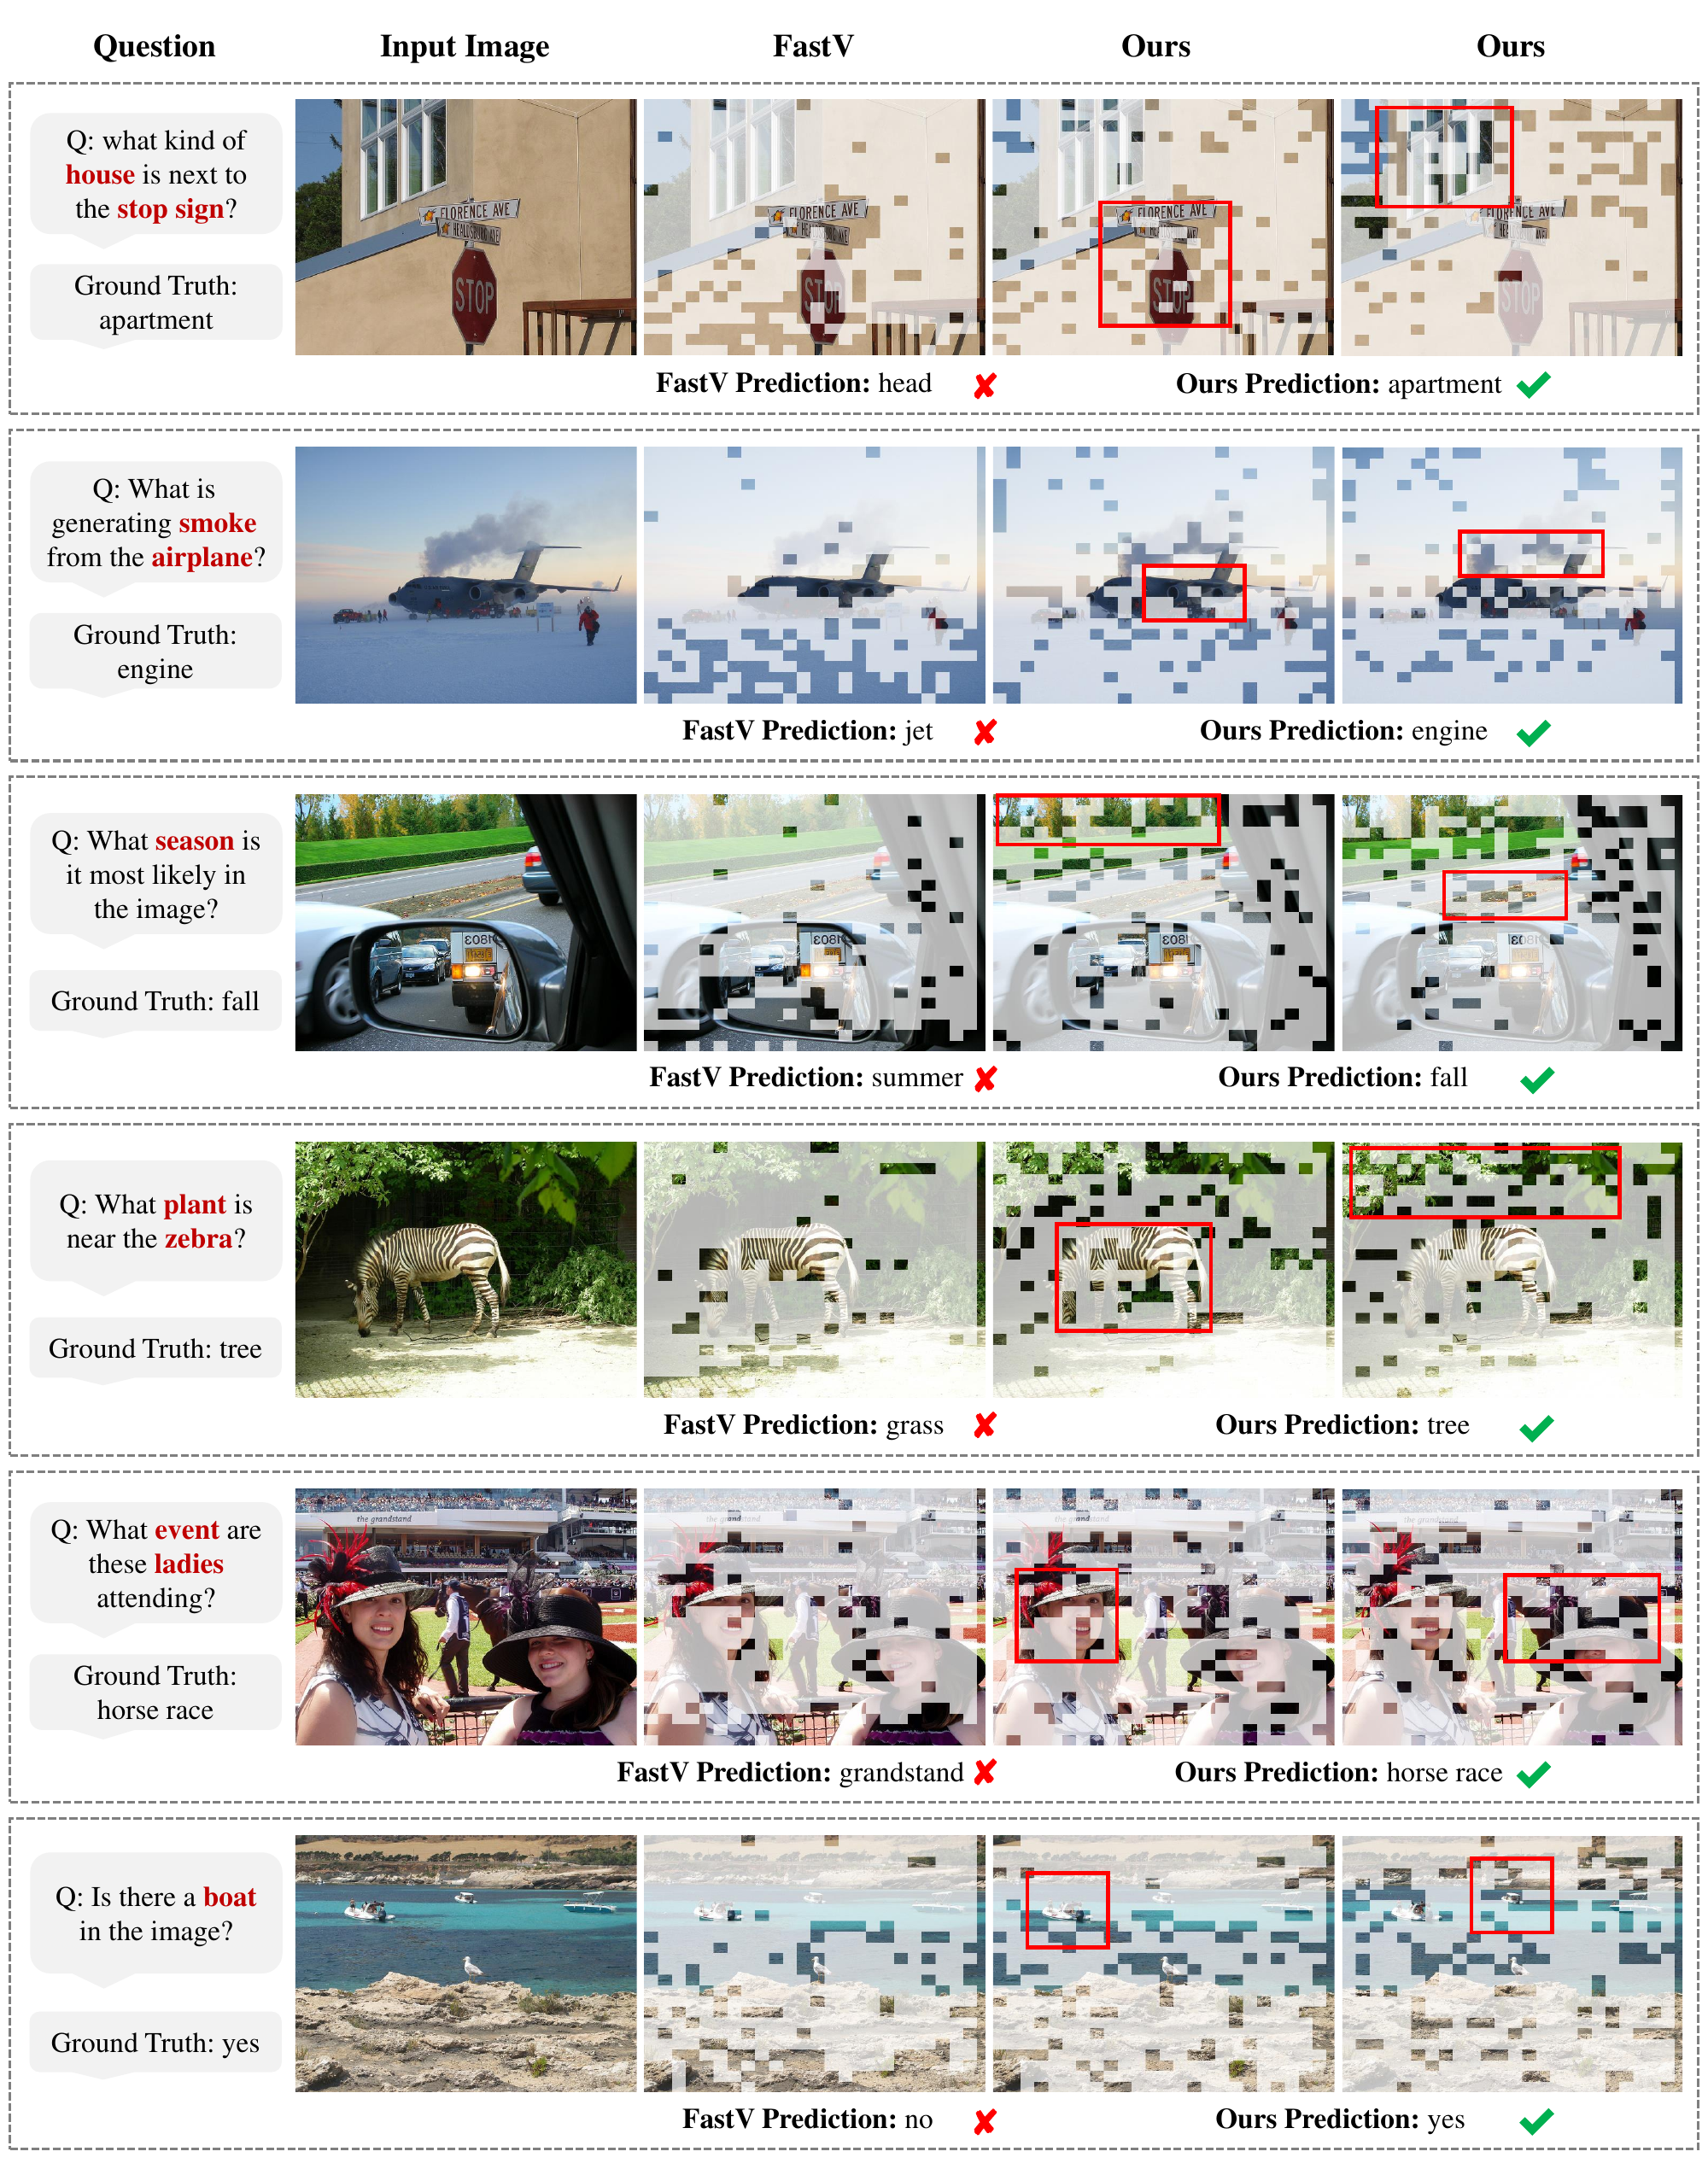}
  \caption{The case comparison between FastV and ALVTS. It presents original images alongside their pruned versions. Grey mask areas indicate discarded tokens. Red bounding boxes highlight key objects referenced in prompts.}
  \label{fig:appendix_visualize}
\end{figure*}
\cref{fig:appendix_visualize} provides additional visualization examples to further illustrate the effectiveness of ALVTS. For each example, we present the token selection results from two different model layers, with red bounding boxes highlighting the key visual regions referenced in the questions. The visualizations show that ALVTS adaptively attends to different image regions across layers, thereby achieving complementary visual information integration. Consider the first image example in the figure, where one layer focuses on the ``stop sign'' while another layer captures the ``house'', both of which are essential for correctly answering the question. In contrast, FastV performs one-time static token pruning at an early layer, and once critical visual regions are discarded, they become permanently inaccessible to all subsequent layers. This irreversible information loss leads to incorrect predictions, as evidenced by FastV's failure on all shown examples. These cases further validate that ALVTS's adaptive layer-wise token selection mechanism effectively preserves essential visual information throughout the model.
