# Supplementary material for: One Layer's Trash is Another Layer's Treasure: Adaptive Layer-wise Visual Token Selection in LVLMs
Source: arXiv:2606.14277 source file (2026-06-12)
Supplement: Supplementary file 2 [file X_suppl_crversion.tex]

\clearpage
\setcounter{page}{1}
\maketitlesupplementary
\appendix  % 自行添加

\section{Benchmark Details}
\label{sec:benchmark details}
\begin{itemize}
\item \textbf{AI2D}~\cite{kembhavi2016diagram} focuses on diagram interpretation and reasoning, comprising over 5,000 grade school science diagrams with comprehensive annotations. Each diagram is associated with multiple-choice questions, totaling more than 15,000 questions across the dataset. This benchmark is specifically designed to evaluate models' ability to understand complex visual structures, parse spatial relationships, and perform domain-specific semantic reasoning about scientific concepts depicted in diagrams.

\item \textbf{POPE}~\cite{li2023evaluating} assesses object hallucination in large vision-language models by formulating evaluation as a binary classification task using simple yes-or-no questions. Built on the MS COCO validation set, we evaluate on 500 randomly selected images with 6 questions per image, totaling 3,000 question-answer pairs. Three sampling strategies are employed: random, popular, and adversarial. The adversarial strategy is particularly critical as it targets objects that frequently co-occur with the ground truth but are not present in the image, thereby rigorously testing the model's tendency to hallucinate based on contextual priors rather than visual evidence. Performance is measured using accuracy, precision, recall, and F1 score.

\item \textbf{TextVQA}~\cite{singh2019towards} addresses visual question answering requiring reading and reasoning about text in images, containing 45,336 questions on 28,408 images sourced from the Open Images dataset. Each question is annotated with 10 human-provided answers, with the dataset split into 34,602 training, 5,000 validation, and 5,734 test questions. Evaluation follows the standard protocol where the predicted answer is compared against 10 human annotations. An answer is considered correct if it matches at least 3 out of 10 human responses. The benchmark tests models' ability to detect, recognize, and reason about textual content embedded within natural scene images. 

\item \textbf{OKVQA}~\cite{marino2019ok} features 14,055 questions where image content alone is insufficient for answering, requiring external knowledge resources. Questions are collected on COCO images, with 9,009 training and 5,046 test samples, each accompanied by 10 answer annotations. The dataset spans 10 knowledge categories including science, history, sports, and geography. We follow the standard evaluation protocol using the VQA accuracy metric, comparing predicted answers against human annotations.

\item \textbf{VizWiz}~\cite{gurari2018vizwiz} is a goal-oriented VQA dataset comprising over 31,000 visual questions from blind users who captured images via mobile phones and recorded spoken queries. Each image is annotated with 10 crowdsourced answers. The dataset presents unique challenges including poor image quality (blur, lighting issues, obstructed views) and conversational question styles. We evaluate on the test split using the standard VQA accuracy metric.

\item \textbf{COCO Caption}~\cite{lin2014microsoft} is built upon the MS COCO dataset, which contains 328,000 images depicting complex everyday scenes with common objects in natural contexts. The dataset comprises 91 object categories and 2.5 million labeled instances. Each image is paired with five human-generated descriptive captions collected via crowdsourcing. Following standard practice, we report CIDEr as the primary captioning metric for performance assessment.

\item \textbf{NoCaps}~\cite{agrawal2019nocaps} is a novel object captioning benchmark consisting of 15,100 images from Open Images with 166,100 human-generated captions. Each image contains 10 reference captions plus one human baseline caption. Test images are divided into in-domain, near-domain, and out-of-domain subsets based on object category overlap with COCO. Specifically, in-domain images contain only objects belonging to COCO classes; near-domain images include a mix of both COCO and novel classes; while out-of-domain images consist exclusively of novel classes. We evaluate on all three splits using the CIDEr metric.

\item \textbf{RealWorldQA} is a real-world visual understanding benchmark containing 765 images captured from vehicles and diverse real-world settings. Each image is paired with a question requiring visual reasoning and a verifiable answer. Questions span object recognition, spatial relationships, directional understanding, and scene comprehension. We report accuracy on the full test set.
\end{itemize}

% ------------------------------
\section{Implementation Details}
Experiments with LLaVA-1.5-7B~\cite{liu2024improved}, LLaVA-NeXT-7B~\cite{liu2024llavanext}, and Qwen2.5-VL-3B-Instruct~\cite{bai2025qwen2} models are conducted on a single NVIDIA GeForce RTX 4090 GPU. Experiments with the LLaVA-1.5-13B model are conducted on a single NVIDIA A100-40G GPU. The implementation is carried out in Python
3.10, utilizing PyTorch 2.1.2 and CUDA 12.2. The inference follows the evaluation settings of the LMMs-Eval framework~\cite{zhang2025lmms}.

% ------------------------------
\section{LLaVA-1.5-13B Detailed Results}
% 表格
\begin{table*}[t]
    \caption{Performance comparison of LLaVA-1.5-13B under different token reduction ratios. ``Avg.'' refers to the average performance across 8 benchmarks. Best results are shown in \textbf{bold}.}
    \label{tab:crversion_appendix_13b}
    
    \centering
    \begin{tabular*}{\textwidth}{@{\extracolsep{\fill}} l|cccccccc|c}
    \toprule
    \textbf{Method} & \textbf{AI2D} & \textbf{POPE} & \textbf{VQA}$^{\text{Text}}$ & \textbf{OKVQA} & \textbf{VizWiz} & \textbf{COCO} & \textbf{NoCaps} & \textbf{RealWorld} & \textbf{Avg.} \\
    \midrule
    \multicolumn{10}{c}{\textit{Upper Bound, 576 Tokens (100\%)}} \\
    \midrule
    LLaVA-1.5-13B & 59.26 & 85.92 & 61.26 & 58.24 & 56.60 & 115.48 & 109.32 & 55.29 & 100.00\% \\
    \midrule
    \multicolumn{10}{c}{\textit{Retain 192 Tokens ($\downarrow$ 67\%)}} \\
    \midrule
    FastV {\footnotesize\textit{(ECCV-24)}} & 58.61 & 82.68 & 60.52 & 56.89 & 57.05 & 114.61 & 107.96 & 54.90 & 98.71\% \\
    VTW {\footnotesize\textit{(AAAI-25)}} & 59.42 & 82.24 & 54.69 & 44.76 & 50.66 & 82.40 & 67.05 & 53.73 & 85.19\% \\
    PDrop {\footnotesize\textit{(CVPR-25)}} & 57.64 & 84.77 & 59.46 & 58.11 & 55.65 & 113.76 & 107.08 & 52.81 & 97.88\% \\
    DART {\footnotesize\textit{(EMNLP-25)}} & 58.94 & 84.02 & 60.16 & 57.13 & \textbf{57.28} & 115.19 & 108.53 & \textbf{55.03} & 99.16\% \\
    \textbf{ALVTS (\textit{Ours})} & \textbf{59.52} & \textbf{85.79} & \textbf{60.62} & \textbf{58.12} & 56.61 & \textbf{116.19} & \textbf{108.96} & \textbf{55.03} & \textbf{99.86\%} \\
    \midrule
    \multicolumn{10}{c}{\textit{Retain 128 Tokens ($\downarrow$ 78\%)}} \\
    \midrule
    FastV {\footnotesize\textit{(ECCV-24)}} & 57.71 & 77.90 & 59.61 & 55.70 & \textbf{57.35} & 112.24 & 105.99 & 52.42 & 96.41\% \\
    VTW {\footnotesize\textit{(AAAI-25)}} & 58.45 & 67.39 & 51.40 & 32.88 & 49.83 & 44.95 & 27.03 & 46.67 & 69.19\% \\
    PDrop {\footnotesize\textit{(CVPR-25)}} & 58.06 & 85.28 & 59.52 & \textbf{57.95} & 53.42 & 110.81 & 102.70 & 52.16 & 96.56\% \\
    DART {\footnotesize\textit{(EMNLP-25)}} & 58.81 & 81.71 & 59.03 & 55.77 & \textbf{57.35} & 112.88 & 106.62 & 53.20 & 97.41\% \\
    \textbf{ALVTS (\textit{Ours})} & \textbf{59.03} & \textbf{86.40} & \textbf{60.49} & 57.75 & 56.77 & \textbf{113.37} & \textbf{106.93} & \textbf{54.51} & \textbf{99.12\%} \\
    \midrule
    \multicolumn{10}{c}{\textit{Retain 64 Tokens ($\downarrow$ 89\%)}} \\
    \midrule
    FastV {\footnotesize\textit{(ECCV-24)}} & 57.74 & 69.32 & 56.16 & 52.01 & \textbf{57.35} & 103.64 & 96.65 & 50.33 & 91.20\% \\
    VTW {\footnotesize\textit{(AAAI-25)}} & 55.70 & 1.46 & 45.16 & 22.83 & 49.98 & 7.80 & 5.08 & 43.40 & 48.35\% \\
    PDrop {\footnotesize\textit{(CVPR-25)}} & 56.87 & 79.83 & 58.00 & 55.38 & 53.46 & 106.92 & 93.99 & 49.54 & 92.66\% \\
    DART {\footnotesize\textit{(EMNLP-25)}} & 57.61 & 75.52 & 55.90 & 52.70 & 57.25 & 108.44 & 102.16 & 53.33 & 93.98\% \\
    \textbf{ALVTS (\textit{Ours})} & \textbf{58.61} & \textbf{82.39} & \textbf{59.18} & \textbf{56.49} & 56.13 & \textbf{109.58} & \textbf{102.66} & \textbf{53.46} & \textbf{96.63\%} \\
    \bottomrule
    \end{tabular*}
\end{table*}
% 设置表格宽度等于文本行宽度
\begin{table*}[t]
    \caption{Ablation study on token selector rank in LLaVA-1.5-7B. Avg. denotes the average performance across all benchmarks relative to the original model, and Overhead indicates the parameter overhead per decoder layer.}
    \label{tab:crversion_appendix_rank_choice}

    % 将表格内所有字体缩小一号
    % \small
    % 稍微减小列间距，为内容和竖线腾出空间
    % \setlength{\tabcolsep}{3pt}

    \begin{tabular*}{\textwidth}{@{\extracolsep{\fill}} ccccccc}
    \toprule
    \textbf{Rank} & \textbf{POPE} & \textbf{OKVQA} & \textbf{COCO} & \textbf{NoCaps} & \textbf{Avg.} & \textbf{Overhead} \\
    \midrule
    32 & 79.10 & 47.87 & 101.51 & 94.08 & 90.67\% & 0.26\% \\
    64 & 81.68 & 48.33 & 105.73 & 95.50 & 92.93\% & 0.52\% \\
    128 & 83.38 & 48.57 & 106.33 & 96.17 & 93.83\% & 1.04\% \\
    256 & 83.87 & 49.66 & 105.89 & 97.60 & 94.72\% & 2.07\% \\
    384 & 84.07 & 49.77 & 106.64 & 97.38 & 94.95\% & 3.11\% \\
    512 & 84.34 & 50.13 & 106.46 & 97.80 & 95.26\% & 4.15\% \\ 
    \bottomrule
    \end{tabular*}
\end{table*}
% 改成跨双栏的排版
\cref{tab:crversion_appendix_13b} presents the detailed per-benchmark performance of LLaVA-1.5-13B under different token reduction ratios. At a 67\% reduction ratio, ALVTS attains 99.86\% average performance, outperforming all competing methods. Notably, ALVTS maintains robust performance even at an 89\% reduction ratio, achieving 96.63\% versus 91.20\% for FastV~\cite{chen2024image}. The method demonstrates particular strength on challenging benchmarks like COCO Caption and NoCaps, validating its effectiveness in preserving critical visual information under aggressive compression.

% ------------------------------
\section{Ablation Study about Token Selector Rank}
To determine the optimal rank for the token selector, we evaluate ALVTS with different rank settings, as shown in \cref{tab:crversion_appendix_rank_choice}. We observe that increasing the rank from 32 to 256 brings notable performance improvements across all benchmarks, lifting the average performance from 90.67\% to 94.72\%. However, further increasing the rank from 256 to 384 yields only marginal gains (94.72\% to 94.95\%), while the parameter overhead per decoder layer increases from 2.07\% to 3.11\%. Therefore, we select a rank of 256 for LLaVA-1.5-7B, as it provides an optimal balance between model performance and parameter efficiency.
