# Supplementary material for: One Layer's Trash is Another Layer's Treasure: Adaptive Layer-wise Visual Token Selection in LVLMs
Source: arXiv:2606.14277 source file (2026-06-12)
Supplement: Supplementary file 4 [file appendix_fastv_dynamic.tex]

\begin{table}[t]
    \caption{Effectiveness of dynamic token selection mechanism on FastV algorithm.}
    \label{tab:appendix_fastv_dynamic}

    \begin{tabular*}{\columnwidth}{@{\extracolsep{\fill}} l|cccc}
    \toprule
    \small\textbf{Method} & \small\textbf{POPE} & \small\textbf{OKVQA} & \small\textbf{COCO} & \small\textbf{NoCaps} \\
    \midrule
    \multicolumn{5}{c}{\textit{Token Reduction ($\downarrow$ 67\%)}} \\
    \midrule
    FastV & 77.79 &	51.77 &	107.49 & 102.26 \\
    FastV \footnotesize(w/ dynamic) & 82.12 &	52.03 &	110.82 & 103.86 \\
    \midrule
    \multicolumn{5}{c}{\textit{Token Reduction ($\downarrow$ 78\%)}} \\
    \midrule
    FastV & 72.10 &	49.90 &	101.99 & 97.06 \\
    FastV \footnotesize(w/ dynamic) & 76.34 &	50.76 &	109.39 & 100.59 \\
    \midrule
    \multicolumn{5}{c}{\textit{Token Reduction ($\downarrow$ 89\%)}} \\
    \midrule
    FastV & 59.55 &	45.14 &	82.62 &	79.01 \\
    FastV \footnotesize(w/ dynamic) & 67.85 &	46.39 &	103.15 & 92.61 \\
    \bottomrule
    \end{tabular*}
\end{table}
