# Supplementary material for: One Layer's Trash is Another Layer's Treasure: Adaptive Layer-wise Visual Token Selection in LVLMs
Source: arXiv:2606.14277 source file (2026-06-12)
Supplement: Supplementary file 5 [file appendix_rank_choice.tex]

\begin{table}[t]
    \caption{Ablation study on token selector rank in LLaVA-1.5-7B. Avg. denotes the average performance across all benchmarks relative to the original model, and Overhead indicates the parameter overhead per decoder layer.}
    \label{tab:appendix_rank_choice}

    % 将表格内所有字体缩小一号
    \small
    % 稍微减小列间距，为内容和竖线腾出空间
    \setlength{\tabcolsep}{3pt}

    \begin{tabular*}{\columnwidth}{@{\extracolsep{\fill}} c|cccccc}
    \toprule
    \textbf{Rank} & \textbf{POPE} & \textbf{OKVQA} & \textbf{COCO} & \textbf{NoCaps} & \textbf{Avg.} & \textbf{Overhead} \\
    \midrule
    64 & 81.68 & 48.33 & 105.73 & 95.50 & 92.93\% & 0.5\% \\
    128 & 83.38 & 48.57 & 106.33 & 96.17 & 93.83\% & 1.0\% \\
    256 & 83.87 & 49.66 & 105.89 & 97.60 & 94.72\% & 2.0\% \\
    384 & 84.07 & 49.77 & 106.64 & 97.38 & 94.95\% & 3.0\% \\
    \bottomrule
    \end{tabular*}
\end{table}
